# Supplementary material for: Reactive near-field subwavelength microwave imaging with a non-invasive Rydberg probe
Source: arXiv:2512.19116 source file (2025-12-22)
Supplement: Supplementary file 2 [file si_bibcite.tex]

% arXiv-safe citation definitions for Supplementary_Information.tex
% This file is input at the start of the SI to ensure citations resolve on arXiv.
% We use S-prefixed labels (S1–S3) consistently in both in-text citations and the SI reference list.

\bibcite{S1}{{S1}{2001}{Lacomme et~al.}{}}
\bibcite{S2}{{S2}{2008}{Vinetti}{}}
\bibcite{S3}{{S3}{2004}{Wang et~al.}{}}
